# Supplementary material for: Deterministic and Probabilistic Error Bounds for Floating Point Summation Algorithms
Source: arXiv:2107.01604 source file (2021-07-04)
Supplement: Supplementary file 1 [file Appendix.tex]

\appendix

\section{Proof of Theorem~\ref{t_cs4}}
We present the proof ideas for the two expressions.

\subsection{First expression}
Abbreviate $a_j\equiv \hat{c}_j{(1+\eta_{j+1})}$ and $b_j\equiv s_j\sigma_j$.
Then $e_2=b_2$ implies
\begin{equation*}
e_3=(e_2-a_2)(1+\sigma_3) +b_3=(b_2-a_2)(1+\sigma_3)+b_3.
\end{equation*}
and
\begin{eqnarray*}
e_4&=&(e_3-a_3)(1+\sigma_4) +x_4\eta_4(1+\sigma_4) +b_4 \\
&=&\left((b_2-a_2)(1+\sigma_3)+(b_3 -a_3)\right)(1+\sigma_4) +x_4\eta_4(1+\sigma_4)+b_4\\
&=&(b_2-a_2)(1+\sigma_3)(1+\sigma_4)+(b_3 -a_3)(1+\sigma_4) +b_4+x_4\eta_4(1+\sigma_4).
\end{eqnarray*}

\subsection{Second expression}
With the assumptions (\ref{e_model1}) abbreviate
\begin{align}\label{e_def}
\begin{split}
X_k&\equiv\sum_{j=2}^k{x_j(\eta_j-\delta_j)\prod_{\ell=j}^k{(1+\beta_{\ell})(1+\eta_{\ell+1})}},
\qquad 2\leq k\leq n-1\\
\Theta_k &\equiv 1-(1+\delta_k)(1+\beta_k)(1+\eta_{k+1}) \qquad 2\leq k\leq n-1\\
E_k&\equiv  e_k\Theta_k+\sum_{j=2}^{k-1}{e_j(\Theta_j+
\delta_{j+1})\prod_{\ell=j+1}^k{(1+\beta_{\ell})(1+\eta_{\ell+1})}}, \qquad 2\leq k\leq n-1.
\end{split}
\end{align}

We look at the first five errors.
\begin{enumerate}
\item Second error:  $e_2=s_2\sigma_2$.
From $a_2=\hat{c}_2(1+\eta_3)$ follows
\begin{eqnarray*}
e_2-a_2&=&\left(e_2-((e_2-e_1)(1+\delta_2)+x_2(\delta_2-\eta_2))\right)(1+\beta_2)(1+\eta_3)\\
&=&e_2\underbrace{\left(1-(1+\delta_2)(1+\beta_2)(1+\eta_3)\right)}_{\Theta_2}
 +\underbrace{x_2(\eta_2-\delta_2)(1+\beta_2)(1+\eta_3)}_{X_2}\\
&=& e_2 \Theta_2+X_2=E_2+X_2.
\end{eqnarray*}

\item Third error: Substitute the above expression for $e_2-a_2$ into the third error
\begin{eqnarray*}
e_3&=&(e_2-a_2)(1+\sigma_3)+x_3\eta_3(1+\sigma_3)+s_3\sigma_3\\
&=&E_2(1+\sigma_3)+\left(x_3\eta_3+X_2\right)(1+\sigma_3)+s_3\sigma_3
\end{eqnarray*}
With $a_3=\hat{c}_3(1+\eta_4)$ we get
\begin{eqnarray*}
e_3-a_3&=&e_3-\left((e_3-e_2)(1+\delta_3)+a_2\right)(1+\beta_3)(1+\eta_4)\\
&&\qquad -x_3(\delta_3-\eta_3)(1+\beta_3)(1+\eta_4)\\
&=&e_3\underbrace{\left(1-(1+\delta_3)(1+\beta_3)(1+\eta_4)\right)}_{\Theta_3}\\
&&\qquad+\left(e_2\delta_3+(e_2-a_2)\right)(1+\beta_3)(1+\eta_4)\\
&&\qquad+x_3(\eta_3-\delta_3)(1+\beta_3)(1+\eta_4).
\end{eqnarray*}
The second error implies for the second term
\begin{equation*}
e_2\delta_3+(e_2-a_2)=e_2\delta_3+e_2\Theta_2+X_2=e_2\delta_3+E_2+X_2
\end{equation*}
Substitute this into $e_3-a_3$,
\begin{eqnarray*}
e_3-a_3&=&\underbrace{e_3\Theta_3+(e_2\delta_3+E_2)(1+\beta_3)(1+\eta_4)}_{E_3}
+X_3=E_3+X_3.
\end{eqnarray*}

 \item Fourth error:
 Substitute the above expression for $e_3-a_3$ into the third error
 \begin{eqnarray*}
e_4&=&(e_3-a_3)(1+\sigma_4)+x_4\eta_4(1+\sigma_4)+s_4\sigma_4\\
&=&E_3(1+\sigma_4)+(x_4\eta_4+X_3)(1+\sigma_4)+s_4\sigma_4.
\end{eqnarray*}
With $a_4=\hat{c}_4(1+\eta_5)$ we get
\begin{eqnarray*}
e_4-a_4&=&e_4-\left((e_4-e_3)(1+\delta_4)+a_3\right)(1+\beta_4)(1+\eta_5)\\
&&\qquad-x_3(\delta_3-\eta_3)(1+\beta_3)(1+\eta_4)\\
&=&e_4\underbrace{\left(1-(1+\delta_4)(1+\beta_4)(1+\eta_5)\right)}_{\Theta_4}\\
&&\qquad +\left(e_3\delta_4+(e_3-a_3)\right)(1+\beta_4)(1+\eta_5)\\
&& \qquad+x_4(\eta_4-\delta_4)(1+\beta_4)(1+\eta_5).
\end{eqnarray*}
The third error implies for the second term
\begin{equation*}
e_3\delta_4+(e_3-a_3)=e_3\delta_4+E_3+X_3.
\end{equation*}
Substitute this into $e_4-a_4$,
\begin{equation*}
e_4-a_4=\underbrace{e_4\Theta_4+(e_3\delta_4+E_3)(1+\beta_4)(1+\eta_5)}_{E_4}+X_4
=E_4+X_4
\end{equation*}

 \item Fifth error:
 Substitute the above expression for $e_4-a_4$ into the third error
 \begin{eqnarray*}
e_5&=&(e_4-a_4)(1+\sigma_5)+x_5\eta_5(1+\sigma_5)+s_5\sigma_5\\
&=&E_4(1+\sigma_5)+(x_5\eta_5+X_4)(1+\sigma_5)+s_5\sigma_5.
\end{eqnarray*}

\item Last error:
\begin{equation*}
e_n= E_{n-1}(1+\sigma_n)+(x_n\eta_n(1+\beta_n) +X_{n-1})(1+\sigma_n)+s_n\sigma_n\\
\end{equation*}
\end{enumerate}
